# Supplementary material for: Phase flip code with semiconductor spin qubits
Source: arXiv:2202.11530 ancillary file (2022-02-23)
Supplement: Supplementary file 1 [file Supplementary_Information.pdf]

# Phase flip code with semiconductor spin qubits: Supplementary Information

F. van Riggelen,[1] W. I. L. Lawrie,[1] M. Russ,[1] N. W. Hendrickx,[1] A. Sammak,[2]
M. Rispler,[3,4] B. M. Terhal,[3,4,5] G. Scappucci,[1] and M. Veldhorst[1,*]

[1] *QuTech and Kavli Institute of Nanoscience, Delft University of Technology, Lorentzweg 1, 2628 CJ Delft, The Netherlands*
[2] *QuTech and Netherlands Organization for Applied Scientific Research (TNO), Stieltjesweg 1 2628 CK Delft, The Netherlands*
[3] *QuTech, Delft University of Technology, Lorentzweg 1, 2628 CJ Delft, The Netherlands*
[4] *JARA Institute for Quantum Information, Forschungszentrum Jülich GmbH, 52428 Jülich, Germany*
[5] *EEMCS, Delft University of Technology, Mekelweg 4, 2628 CD Delft, The Netherlands*

* m.veldhorst@tudelft.nl

# I. SPIN READOUT BASED ON PAULI SPIN BLOCKADE

In this work we make use of the same latched PSB protocol as used in previous works [1, 2]. The aim is to reduce the readout infidelity which results from spin relaxation due to spin-orbit interaction [3, 4]. The tunneling rates from the quantum dots to the reservoir are tuned to be asymmetrical, resulting in a high tunneling rate for the (1,1)-(0,1) charge transition and a low tunneling rate for the (1,1)-(1,2) charge transition, as depicted in Figure S1a. For the readout we pulse from (1,1) to a spot in the (0,2) charge regime that is bounded by the extension of the (1,1)-(0,1) and (1,1)-(1,2) charge transition lines. When the transition to the (0,2) state is blocked, the (0,1) state is accessible and one hole will tunnel to the reservoir. Since the decay to the (0,2) state from the (0,1) state is determined by the slow tunneling rate, the system is now locked in a metastable charge state, thereby enabling spin-to-charge conversion. We use this readout method on two pair of qubits, Q1 and Q2, using S1 as charge sensor (called readout system Q1Q2), and Q3 and Q4, using S2 as charge sensor (called readout system Q3Q4). Each sensor can measure both pairs of qubits, however it is more sensitive to the quantum dots that are closest. We operate in the regime where the $|{\downarrow\downarrow}\rangle$ state is blocked and the other spin states are (partially) non-blocked, as shown in Figure S1c,e. Therefore, this readout method can only be used to determine the spin state of one of the qubits in the readout pair when the state of the other qubit is $|{\downarrow}\rangle$. The Q3Q4 readout system is used in the final three-qubit phase flip experiment described in the main text. The fraction of tunneling that is blocked for the different spin states influences how well we can read out the final results of this experiment. If the desired output state is $|{\downarrow\downarrow}\rangle$ (as for no errors or a single error), any error will give a different readout result. However, if the desired output state is $|{\downarrow\uparrow}\rangle$ (as for two or three errors), an error is very hard to detect. This is what we call asymmetry in the readout. The effect of the readout in combination with the SWAP gate is described in more detail in Supplementary Information VII.

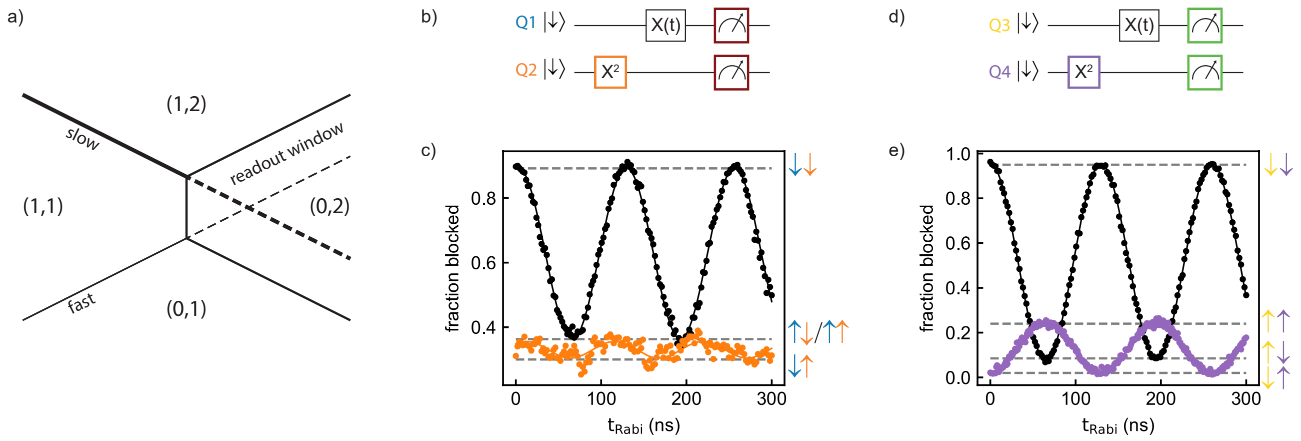


Figure S1. **Fraction of the tunneling that is blocked per spin state** (a) Schematic drawing of the charge stability diagram showing the (1,1)-(0,2) anticrossing and indicating the readout window. (b) Circuit diagram describing the experiment to map out the fraction of the tunneling that is blocked per spin state in the two-qubit subspace of the Q1Q2 readout system [5]. A Rabi experiment is performed on Q1 with Q2 either in the $|{\downarrow}\rangle$ (without the $X^2$ on Q2, indicated with the orange box) or $|{\uparrow}\rangle$ state (with the $X^2$ on Q2). (c) Results of the experiment described in (b). The black data points correspond to the Rabi experiment with Q2 in the $|{\downarrow}\rangle$ state and the orange data points to the experiment with Q2 in the $|{\uparrow}\rangle$ state. It shows that there is good contrast between the $|{\downarrow\downarrow}\rangle$ state and the anti-parallel states, but the $|{\uparrow\uparrow}\rangle$ state can hardly be distinguished from the anti-parallel states. (d) Circuit diagram describing the same experiment as in (b), but for the Q3Q4 readout system. (e) Shown are the results of the experiment as described in (d). For the Rabi experiment performed on Q3 with Q4 in the $|{\downarrow}\rangle$ state, the data is plotted in black, with Q4 in the $|{\uparrow}\rangle$ state, the data is plotted in purple. It becomes apparent that also for this readout system there is a clear contrast between $|{\downarrow\downarrow}\rangle$ and both anti-parallel spin states. The $|{\uparrow\uparrow}\rangle$ state however is partially blocked.

## II. CZ AND CS$^{-1}$ GATE CALIBRATION

The CZ and CS$^{-1}$ gates are calibrated using a Ramsey type experiment in which $P_{up}$ is measured as a function of the phase Z($\varphi$) before the final X gate. Overall we follow the same strategy for the calibration as in previous work [1]. For the CS$^{-1}$ gate the circuit diagram of this sequence is shown in Figure 3c of the main text. For the CZ between Q4 and Q3 the circuit is shown in Figure S2a, the same experiment was performed with Q1 as control qubit. To calibrate the phase difference between experiments with and without a preparation pulse on the control qubit, the depth and the length of the pulse on the virtual barrier are tuned. The shape of this pulse is a Tukey window, also called a cosine-tapered window [6]. It is a pulse of which the slopes are the shape of a cosine and in the middle it is flat like a rectangle, as shown in Figure S2b. A factor $\alpha$ determines the precise shape of the pulse: the cosine lobe has width $N \cdot \alpha/2$, which is combined with a rectangular window of width $N(1-\alpha/2)$, where $N$ is the length of the pulse. For the CZ and CS$^{-1}$ gates we used $\alpha = 0.83$. We use the Tukey shape to optimize the adiabaticity of the variation in exchange with respect to the difference in Zeeman energy between the qubits. A CZ gate is obtained when the phase difference is $\pi$, for the situation where the control qubit is in the $|\downarrow\rangle$ state compared to when it is in the $|\uparrow\rangle$ state. A CS$^{-1}$ gate is obtained when the difference in acquired phase is -$\pi/2$. For both the calibration of the CZ as for the CS$^{-1}$, after the exchange pulse, a software Z gate is applied to both of the qubits, to compensate for acquired single-qubit phases. The result of these calibrations are shown in the main text, in Figure 1d for the CZ and in Figure 3d for the CS$^{-1}$.

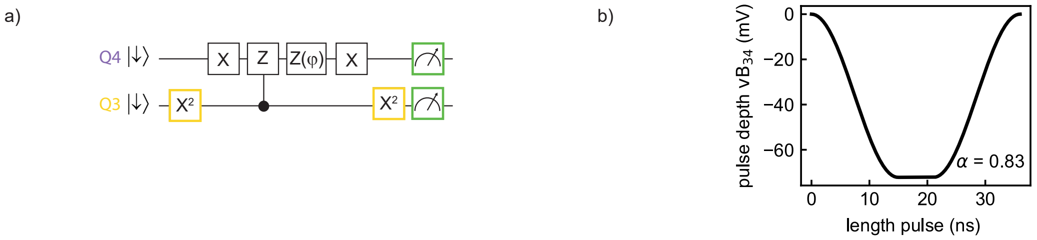


Figure S2. **Calibration and pulse shape CZ and CS$^{-1}$ gates** (a) Circuit diagram of a Ramsey type experiment to measure the conditional phase. This experiment is performed with and without the preparation gate $X^2$ on the control qubit. The conditional-Phase gate is implemented with a pulse on the virtual barrier gate [1] between the two relevant qubits (either gate $vB_{34}$ or $vB_{41}$). The length and depth of this pulse determines the acquired phase and makes a CZ or CS$^{-1}$ gate. (b) Tukey shape with $\alpha = 0.83$ as is used for the implementation of the CZ and CS$^{-1}$ gates. Here we show the pulse with length (36 ns) and depth (-77.2 mV) on the virtual barrier $vB_{34}$ to implement the CZ gate between Q3 and Q4. The depth of the pulse on the virtual barrier is relative to the value it has in the 'exchange off' regime. To implement the CZ (CS$^{-1}$) between Q4 and Q1 a similar pulse is applied to $vB_{41}$ with a length of 34 ns (14 ns) and a depth of -74.6 mV (-73.6 mV).

## III. TWO-QUBIT PHASE FLIP CODE

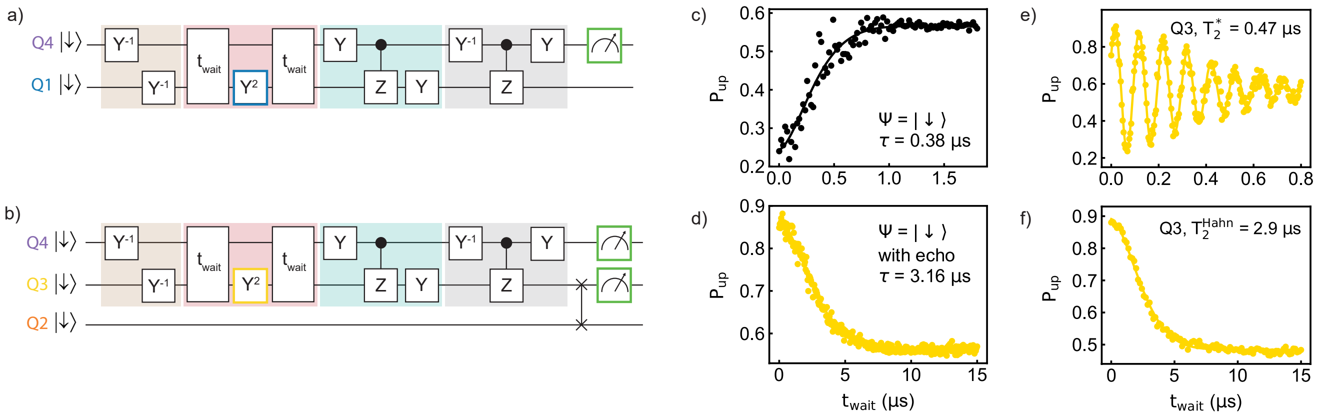


Figure S3. **Two-qubit phase flip code with input state** $|\Psi\rangle = |{\downarrow}\rangle$ (a) Circuit diagram describing the experiment for which the result is shown in Figure 2d of the main text. In this experiment both the data qubit, Q4, and the ancilla qubit, Q1, start in the $|{\downarrow}\rangle$ basis state. For this input state, the logical qubit after the encoding step is $|{-}{-}\rangle$, which is not an entangled state. Therefore, the first CZ gate becomes obsolete and the algorithm can be simplified. An echo pulse is applied to the ancilla qubit (indicated by the blue box), resulting in an experiment that closely resembles a Hahn echo experiment, plus the decoding and correction step. (b) Circuit diagram similar to the one shown in (a), but with Q3 as ancilla qubit. Since the spin state of Q4 is read out with respect to the spin state of Q3, the state of Q3 is reset by applying a resonant SWAP gate between Q3 and Q2. The echo on the ancilla is indicated with a yellow box. (c,d) Plotted here are the spin-up probability as a function of $t_{\mathrm{wait}}$ when executing the circuit diagram in (b), without (c) and with an echo pulse $Y^2$ (d). Individual qubit $T_2^*$ (e) and $T_2^{\mathrm{Hahn}}$ times (f) for Q3.

## IV. SWAP GATE CALIBRATION

To implement a resonant SWAP gate between Q2 and Q3, a Tukey shaped pulse with an oscillation superimposed is applied to the virtual barrier $vB_{23}$, as shown in Figure 3a of the main text. The Tukey shaped pulse is discussed in detail in section II, for the implementation of the SWAP we use $\alpha = 0.5$. To correctly implement the SWAP the length and depth of the Tukey pulse and the AC amplitude and frequency of the oscillation need to be calibrated. We start by choosing the depth of the pulse on $vB_{23}$ as -30 mV compared to the 'exchange off' regime. With this pulse on the virtual barrier we first do a first rough measurement of the difference in resonance frequency between Q2 and Q3. This value we use as the frequency of the oscillation and we vary the length of the SWAP pulse ($t_{SWAP}$) and the AC amplitude (Figure S4a), resulting in the measurement shown in Figure S4b. Based on this measurement we choose a length (80 ns) and AC amplitude (35 mV) of the pulse. As a final step in the calibration, we fine tune the frequency of the oscillation. This we do using the measurement depicted in Figure 3a of the main text, for various values of the frequency and choosing the one where the amplitude measured on Q3 is smallest.

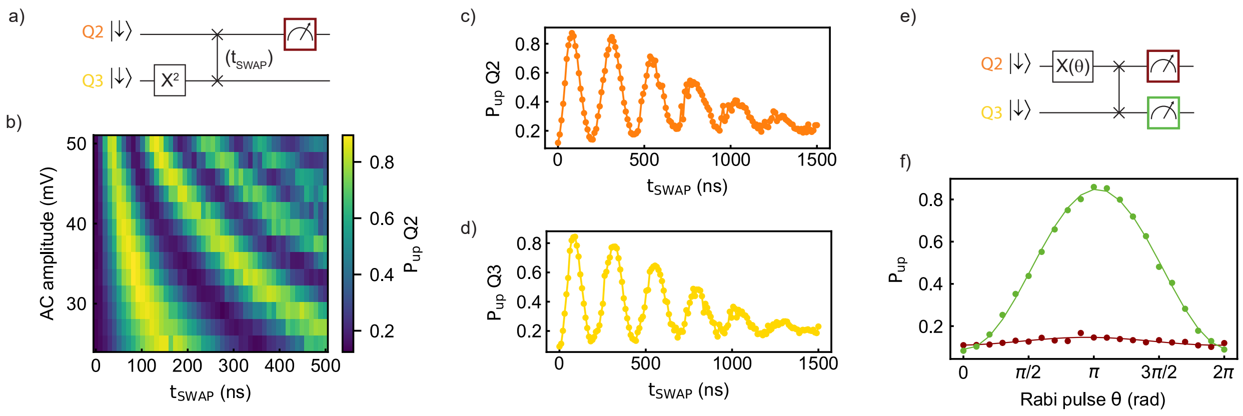


Figure S4. **SWAP gate** (a) Circuit diagram of the experiment used to calibrate the length and AC amplitude of the exchange pulse which implements the resonant SWAP gate. An $X^2$ gate is applied to Q3, after which the SWAP gate is applied and Q2 is read out using the Q1Q2 readout system. (b) Result of the experiment in (a), it shows SWAP oscillations which become faster when the AC amplitude of the exchange pulse is increased [7]. (c, d) Similar experiment as shown in (a), which a fixed value for the AC amplitude of 35 mV. (c) Result of the experiment with an $X^2$ gate on Q3 and using readout system Q1Q2, while (d) shows the result of the same experiment but with an $X^2$ gate on Q2 and using readout system Q3Q4. The decay of the SWAP oscillations is asymmetric, slightly more so for the oscillation shown in (d) than in (c). A possible explanation is that spin states in the qubit partially get swapped with down spins in Q1 and Q4, because the exchange between Q2 and Q1 and between Q3 and Q4 is finite, as shown in section VI. (e) Circuit diagram of an experiment where we put a Rabi oscillation on Q2, swap the states of Q2 and Q3 and read out either with readout system Q1Q2 (red) or Q3Q4 (green). (f) Result of the experiment in (e). It demonstrates that the resonant SWAP gate can also be used to reset Q2, similar to how the SWAP gate can be used to reset Q3, which is shown in Figure 3b of the main text.

## V. TOFFOLI-LIKE GATE

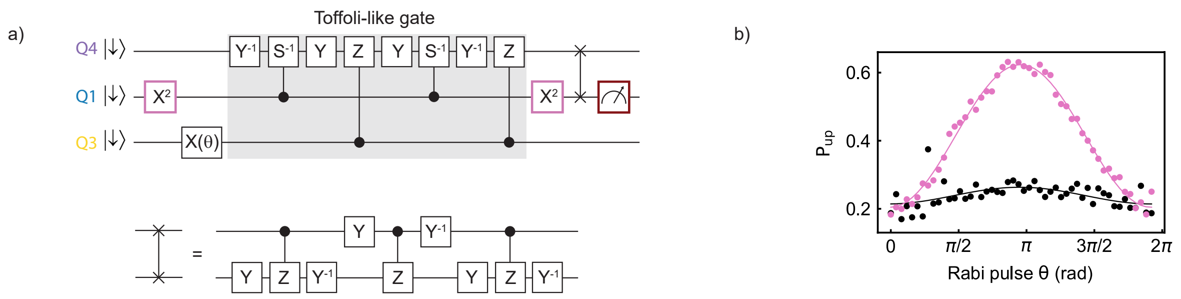


Figure S5. **Toffoli-like gate** (a) Circuit diagram of the Toffoli-like gate composed of CS$^{-1}$ and CZ gates. Before the readout, a SWAP operation is performed between Q4 and Q1. The SWAP gate is composed of three CNOT gates, each one broken down into CZ and Y and Y$^{-1}$ as shown below the circuit diagram. (b) Results of implementing the Toffoli-like gate with target qubit Q4 and control qubits Q1 and Q3. A Rabi oscillation X($\theta$) is applied to Q3 and the final state of Q4 is measured by swapping the state of Q4 with the state of Q1 and using readout system Q1Q2. If ancilla qubit Q1 stays in the $|\downarrow\rangle$ state, the target qubit Q4 also stays in the $|\downarrow\rangle$ state, as plotted in black. However, when Q1 is prepared in the state $|\uparrow\rangle$, Q4 starts to oscillate like Q3, as plotted in pink. With this experiment we demonstrate that the Toffoli-like gate also works for all possible input states of Q3. The overall visibility is smaller compared to the results shown in Figure 3f in the main text, which can be contributed to the SWAP operation, which is composed of multiple gates.

The matrix representation of the circuit diagram of the Toffoli-like gate (see Fig. S5 a) in the basis $\{|\downarrow\rangle_{Q4}, |\uparrow\rangle_{Q4}\} \otimes \{|\downarrow\rangle_{Q1}, |\uparrow\rangle_{Q1}\} \otimes \{|\downarrow\rangle_{Q3}, |\uparrow\rangle_{Q3}\}$ reads

$$\text{Toffoli-like gate} = \begin{pmatrix} 1 & 0 & 0 & 0 & 0 & 0 & 0 & 0 \\ 0 & 1 & 0 & 0 & 0 & 0 & 0 & 0 \\ 0 & 0 & -i & 0 & 0 & 0 & 0 & 0 \\ 0 & 0 & 0 & 0 & 0 & 0 & 0 & 1 \\ 0 & 0 & 0 & 0 & 1 & 0 & 0 & 0 \\ 0 & 0 & 0 & 0 & 0 & 1 & 0 & 0 \\ 0 & 0 & 0 & 0 & 0 & 0 & -i & 0 \\ 0 & 0 & 0 & 1 & 0 & 0 & 0 & 0 \end{pmatrix}. \quad (1)$$

Note, that this matrix corresponds to the real Toffoli-gate up to phases on the two control qubits (here Q1 and Q3) which is irrelevant due to the imminent measurement.

## VI. RESIDUAL EXCHANGE

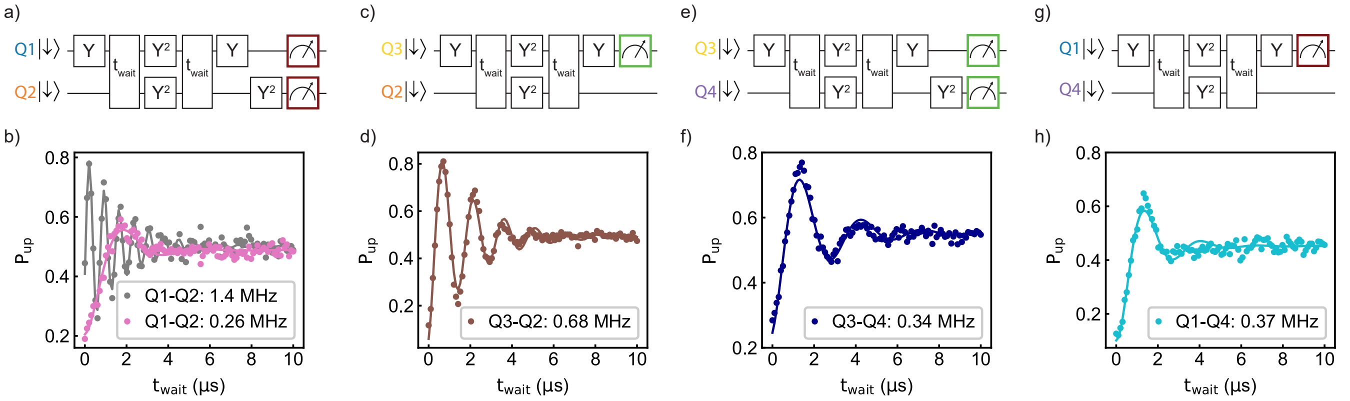


Figure S6. **Residual exchange (or ZZ crosstalk)** (a) Circuit diagram of the measurement of the residual exchange between Q1 and Q2, i.e. the exchange in the regime where the single qubit gates are performed. We execute a Hahn echo experiment on Q1 and apply a $Y^2$ gate on Q4 simultaneous with the echo pulse $Y^2$ on Q1. We measure an oscillation due to the ZZ interaction as a function of $t_{wait}$. (b) Measurement result of the residual exchange between Q1 and Q2. It was first measured to be 1.40 $\pm$ 0.01 MHz (gray). After decreasing the detuning and increasing the voltage on the virtual barrier gate, the exchange was measured again and found to be 0.26 $\pm$ 0.01 MHz (pink). For this qubit pair we chose to reduce the exchange because it was significantly larger than between the other pairs. (c-g) Circuit diagram and results of measurement of the residual exchange between Q3-Q2 (c,d), Q3-Q4 (e,f) and Q1-Q4 (g,h). Values found are 0.68 $\pm$ 0.1 MHz, 0.34 $\pm$ 0.01 MHz and 0.37 $\pm$ 0.01 MHz for Q3-Q2, Q3-Q4 and Q1-Q4 respectively.

## VII. LOGICAL ERROR PROBABILITY FIT FOR THE THREE-QUBIT PHASE FLIP CODE

In this section we derive a model for the three-qubit phase flip code experimentally implemented in the main text and the logical error probability fit function $\Gamma(p)$. For simplicity the implemented gates are assumed to be perfect and are described by their corresponding unitary matrix except for the final SWAP gate. To follow the notation in the main text, we define an X (Y) gate as a $\pi/2$ rotation, $\mathrm{X}^2$ ($\mathrm{Y}^2$) as a $\pi$ rotation and $\mathrm{X}^{-1}$ ($\mathrm{Y}^{-1}$) as a $-\pi/2$ rotation around the $\hat{x}$ ($\hat{y}$) axis. Thus, the unitaries of the single qubit gates read

$$Q = \exp(-i\frac{\pi}{4}\sigma_q) \tag{2}$$

with $Q = X, Y, Z$, $q = x, y, z$, the Pauli matrices $\sigma_q$, and $Q^{-1} = Q^\dagger$ being it's inverse. The unitary of the CZ gate reads

$$\textsc{cz} = \mathrm{diag}(1, 1, 1, -1). \tag{3}$$

Here, we additionally make use of indices to label the affected qubit(s), i.e., $X_{\mathrm{Q1}}$ corresponds to a $X$-gate on Q1 and $\textsc{cz}_{12}$ corresponds on a $\textsc{cz}$-gate between Q1 and Q2.

Moreover, we define the unitary of the two-qubit $\textsc{cs}$ gate as

$$\textsc{cs} = \mathrm{diag}(1, 1, 1, i) \tag{4}$$

and we model an imperfect SWAP gate by the following unitary

$$\textsc{swap}(\epsilon) = \begin{pmatrix} 1 & 0 & 0 & 0 \\ 0 & -i\sqrt{\epsilon}\, e^{\frac{i\pi}{2}\sqrt{1-\epsilon}} & -i\sqrt{1-\epsilon}\, e^{\frac{i\pi}{2}\sqrt{1-\epsilon}} & 0 \\ 0 & -i\sqrt{1-\epsilon}\, e^{\frac{i\pi}{2}\sqrt{1-\epsilon}} & i\sqrt{\epsilon}\, e^{\frac{i\pi}{2}\sqrt{1-\epsilon}} & 0 \\ 0 & 0 & 0 & 1 \end{pmatrix} \tag{5}$$

with an error probability $\epsilon = [0, 1]$. This mimics the time-evolution of a strongly driven resonant-SWAP gate [7]. Note, that strong driving can yield errors similar to off-resonant driving due to non-linear exchange $J \propto \exp\left[2\alpha(v_0 + v_D\cos(2\pi f_D t))\right] \approx \exp(2\alpha v_0)(1 + 2\alpha v_D \cos(2\pi f_D t) + \alpha^2 v_D^2[1 + \cos(4\pi f_D t)])$ causing a shift in the resonance condition. Here, $v_0$ is the voltage setting during the AC drive, $v_D$ is the amplitude of the AC signal, $\alpha$ corresponds to the lever arm of the barrier gate, and $f_D = f_{\mathrm{Q2}} - f_{\mathrm{Q3}}$ is the drive frequency of the AC SWAP gate between Q2 and Q3.

The density matrix $\rho$ after each gate is then given by composing $\rho_1 = U\,\rho_0\,U^\dagger$ with the unitary matrix $U$ chosen from the set above. The uncorrelated probabilistic phase error of each qubit is modelled via the Pauli-Z error channel

$$\Lambda(\rho) = (1 - p)\rho + p\,\sigma_z\,\rho\,\sigma_z \tag{6}$$

applied on each qubit independently with probability $p$. The logical error probability for the three-qubit phase flip code $\Gamma(p)$ is given by the probability to measure $|\Psi\rangle_{\mathrm{Q4}} = |{\downarrow}\rangle$. The probability to measure $|\Psi\rangle_{\mathrm{Q4}} = |{\downarrow}\rangle$ after the PSB measurement of readout system Q3Q4 is given by the positive valued operator (POVM) outcome

$$\Gamma(p) = \mathrm{tr}(\rho_{\mathrm{final}} F_{|\Psi\rangle_{\mathrm{Q4}}=|\downarrow\rangle}) \tag{7}$$

with

$$F_{|\Psi\rangle_{\mathrm{Q4}}=|\downarrow\rangle} = \mathbb{1}_2 \otimes \mathbb{1}_2 \otimes \begin{pmatrix} F_{\downarrow\downarrow} & 0 & 0 & 0 \\ 0 & F_{\downarrow\uparrow} & 0 & 0 \\ 0 & 0 & F_{\uparrow\downarrow} & 0 \\ 0 & 0 & 0 & F_{\uparrow\uparrow} \end{pmatrix} \tag{8}$$

with the same parameters and definitions as above. For an ideal measurement $\Gamma(p) = 1 - 3p^2 + 2p^3$ directly shows the insensitivity of the three-qubit phase code to phase errors by suppressing terms linear in $p$.

Coherent and incoherent unintentional phase errors will provide an additional reduced visibility and an offset of the measurement outcomes which we will account for by introducing the two fitting parameters $a$ and $b$. The final formula to fit our data is then given by plugging in the numbers $F_{\downarrow\downarrow} = 0.95$, $F_{\uparrow\downarrow} = 0.085$, $F_{\downarrow\uparrow} = 0.02$, $F_{\uparrow\uparrow} = 0.24$ in Eq. (7)

$$\Gamma(p) = a\,(0.95 - 1.73\epsilon\, p - 2.79\, p^2 + 3.9\epsilon\, p^2 + 1.86p^3 - 2.17\epsilon\, p^3) + b. \tag{9}$$

The strong suppression of phase errors for an ideal measurement is reduced for a erroneous SWAP-gate $\epsilon > 0$ by not suppressing all linear terms in Eq. (9).

Additionally, the symmetric behavior expected for a theoretical $\Gamma(p)$ under the reflection on the straight line $l(p)$ through points $(p, \Gamma(p)) = (0, a\,F_{\downarrow\downarrow})$ and $(p, \Gamma(p)) = (1, a\,F_{\downarrow\uparrow})$ is broken through the erroneous SWAP-gate [8]. Note, that $(F_{\downarrow\downarrow} - F_{\downarrow\uparrow})$ defines the visibility window of the measurement. This symmetry is given by the fact that the code itself cannot distinguishes between no error ($p = 0$) and an error on all qubits ($p = 1$). We want to note that in our case the imperfect SWAP-gate combined with a finite dark signal ($F_{\downarrow\uparrow} \neq 0$, $F_{\downarrow\uparrow} \neq 0$, $F_{\uparrow\uparrow} \neq 0$ or $F_{\uparrow\uparrow} \neq F_{\downarrow\downarrow}$) of the measurement signal can leave the impression that this symmetry is broken. In short, a single error is detected with a higher contrast $(F_{\downarrow\downarrow} - F_{\downarrow\uparrow})$ than two errors $(F_{\uparrow\uparrow} - F_{\uparrow\downarrow})$ giving rise to a skewing of the signal. As a final remark, there are other errors which give similar correlations than the erroneous SWAP gate. Since these errors cannot be distinguished in the measurement signal, the error probability $\epsilon$ considers all of them and for simplicity are attributed to the dominating SWAP error.

[1] Hendrickx, N. W.; Lawrie, W. I. L.; Russ, M.; van Riggelen, F.; de Snoo, S. L.; Schouten, R. N.; Sammak, A.; Scappucci, G.; Veldhorst, M. A four-qubit germanium quantum processor. *Nature* **2021**, *591*, 580–585.

[2] Lawrie, W. I. L.; Russ, M.; van Riggelen, F.; Hendrickx, N. W.; de Snoo, S. L.; Sammak, A.; Scappucci, G.; Veldhorst, M. Simultaneous driving of semiconductor spin qubits at the fault-tolerant threshold. *arXiv:2109.07837 [cond-mat]* **2021**, arXiv: 2109.07837.

[3] Hendrickx, N. W.; Lawrie, W. I. L.; Petit, L.; Sammak, A.; Scappucci, G.; Veldhorst, M. A single-hole spin qubit. *Nature Communications* **2020**, *11*, 3478.

[4] Danon, J.; Nazarov, Y. V. Pauli spin blockade in the presence of strong spin-orbit coupling. *Physical Review B* **2009**, *80*, 041301.

[5] Lawrie, W. I. L. et al. Quantum dot arrays in silicon and germanium. *Applied Physics Letters* **2020**, *116*, 080501.

[6] Harris, F. On the use of windows for harmonic analysis with the discrete Fourier transform. *Proceedings of the IEEE* **1978**, *66*, 51–83.

[7] Sigillito, A. J.; Gullans, M. J.; Edge, L. F.; Borselli, M.; Petta, J. R. Coherent transfer of quantum information in a silicon double quantum dot using resonant SWAP gates. *npj Quantum Information* **2019**, *5*, 110.

[8] Cramer, J.; Kalb, N.; Rol, M. A.; Hensen, B.; Blok, M. S.; Markham, M.; Twitchen, D. J.; Hanson, R.; Taminiau, T. H. Repeated quantum error correction on a continuously encoded qubit by real-time feedback. *Nature Communications* **2016**, *7*, 11526.
